# Supplementary material for: Universal Marginalizer for Amortised Inference and Embedding of Generative Models
Source: arXiv:1811.04727 source file (2018-11-12)
Supplement: Supplementary file 1 [file appendix.tex]

\appendix

\newpage
\section{Additional Results}
\label{section:additional_results}

\begin{table}[h]
  \caption{Effective sample size for hybrid UM-IS scheme with 2 million samples}
  \label{table:ess}
  \centering
  \begin{tabular}{cllllll}
    \toprule
     $\boldsymbol{\beta}$ & $0.0$ & $0.1$ & $0.25$ & $0.5$ & $0.75$ & $1.0$ \\
    \midrule
    \textbf{ESS} & 7678 & 15458 & 11779 & 1218 & 171 & 92 \\
    \bottomrule
  \end{tabular}
\end{table}
